# Supplementary material for: Magnetoelastic mapping of the high-field phase diagram in the topological cubic helimagnet SrFeO$_{3}$
Source: arXiv:2605.22517 source file (2026-06-14)
Supplement: Supplementary file 1 [file SrFeO3_supple.tex]

\documentclass[reprint,superscriptaddress,aps]{revtex4-1}
\usepackage{amsmath}
\usepackage{amssymb}
\usepackage{bm}
\usepackage{braket}
\usepackage{color}
\usepackage[varg]{txfonts}
\usepackage{varwidth}
\usepackage{dcolumn}
\usepackage[breaklinks,colorlinks=true,linkcolor=blue,urlcolor=cyan,citecolor=blue]{hyperref}
\usepackage{amsmath}

\usepackage{here}
\usepackage[dvipdfmx]{graphicx}

\begin{document}

\title{Supplemental Material for\\``Magnetoelastic mapping of the high-field phase diagram in the topological cubic helimagnet SrFeO$_{3}$"}

\author{Masaki~Gen}
\email{gen@issp.u-tokyo.ac.jp}
\affiliation{Institute for Solid State Physics, University of Tokyo, Kashiwa 277-8581, Japan}
\affiliation{RIKEN Center for Emergent Matter Science (CEMS), Wako 351-0198, Japan}

\author{Shun~Okumura}
\email{okumura@ap.t.u-tokyo.ac.jp}
\affiliation{RIKEN Center for Emergent Matter Science (CEMS), Wako 351-0198, Japan}
\affiliation{Quantum-Phase Electronics Center, The University of Tokyo, Tokyo 113-8656, Japan}
\affiliation{International Institute for Sustainability with Knotted Chiral Meta Matter (WPI-SKCM$^2$),
Hiroshima University, Hiroshima 739-8531, Japan}

\author{Shusaku~Imajo}
\affiliation{Institute for Solid State Physics, University of Tokyo, Kashiwa 277-8581, Japan}
\affiliation{Department of Advanced Materials Science, The University of Tokyo, Kashiwa 277-8561, Japan}

\author{Taro~Nakajima}
\affiliation{Institute for Solid State Physics, University of Tokyo, Kashiwa 277-8581, Japan}
\affiliation{RIKEN Center for Emergent Matter Science (CEMS), Wako 351-0198, Japan}
\affiliation{Institute of Materials Structure Science, High Energy Accelerator Research Organization, Tsukuba 305-0801, Japan}

\author{Karel~Prokes}
\affiliation{Helmholtz-Zentrum Berlin f\"{u}r Materialien und Energie, Hahn-Meitner Platz 1, 14109 Berlin, Germany}

\author{Shunsuke~Kitou}
\affiliation{Department of Advanced Materials Science, The University of Tokyo, Kashiwa 277-8561, Japan}

\author{Yusuke~Tokunaga}
\affiliation{Department of Advanced Materials Science, The University of Tokyo, Kashiwa 277-8561, Japan}

\author{Yoichi~Nii}
\affiliation{Department of Applied Physics and Physico-Informatics, Faculty of Science and Technology, Keio University, Yokohama 223-8522, Japan}

\author{Koichi~Kindo}
\affiliation{Institute for Solid State Physics, University of Tokyo, Kashiwa 277-8581, Japan}

\author{Yoshimitsu~Kohama}
\affiliation{Institute for Solid State Physics, University of Tokyo, Kashiwa 277-8581, Japan}

\author{Shintaro~Ishiwata}
\affiliation{Division of Materials Physics, Graduate School of Engineering Science, The University of Osaka, Osaka 560-8531, Japan}

\author{Taka-hisa~Arima}
\affiliation{RIKEN Center for Emergent Matter Science (CEMS), Wako 351-0198, Japan}
\affiliation{Department of Advanced Materials Science, The University of Tokyo, Kashiwa 277-8561, Japan}

\maketitle
%%%%%%%%%%%%%%%%%%%%%%%%%%%%%%%%%%%%%%%%%%%%%%%%%%%%%%%%

\onecolumngrid

\vspace{+1.5cm}
This Supplemental Material includes contents as listed below:\\
\\
Note 1.~Additional magnetization data in pulsed high magnetic fields\\
Note 2.~Additional magnetostriction data in pulsed high magnetic fields\\
Note 3.~Additional ultrasound data in pulsed high magnetic fields\\
Note 4.~Additional neutron scattering data under tilted magnetic fields\\
Note 5.~Magnetic structure of 4{\it Q}-IFC phase\\

\newpage
\subsection*{\label{Sec1} \large Note 1.~Additional magnetization data in pulsed high magnetic fields}
\vspace{+0.2cm}

Figure~\ref{FigS1} compares the magnetization data for $H \parallel [111]$ and $H \parallel [001]$, which are used to construct the $H$--$T$ phase diagram shown in Fig.~1(c) of the main text.
The data in Figs.~\ref{FigS1}(a) and \ref{FigS1}(b) are identical to those in Fig.~3(a) of the main text.

\begin{figure*}[h]
\centering
\vspace{+1.0cm}
\includegraphics[width=\linewidth]{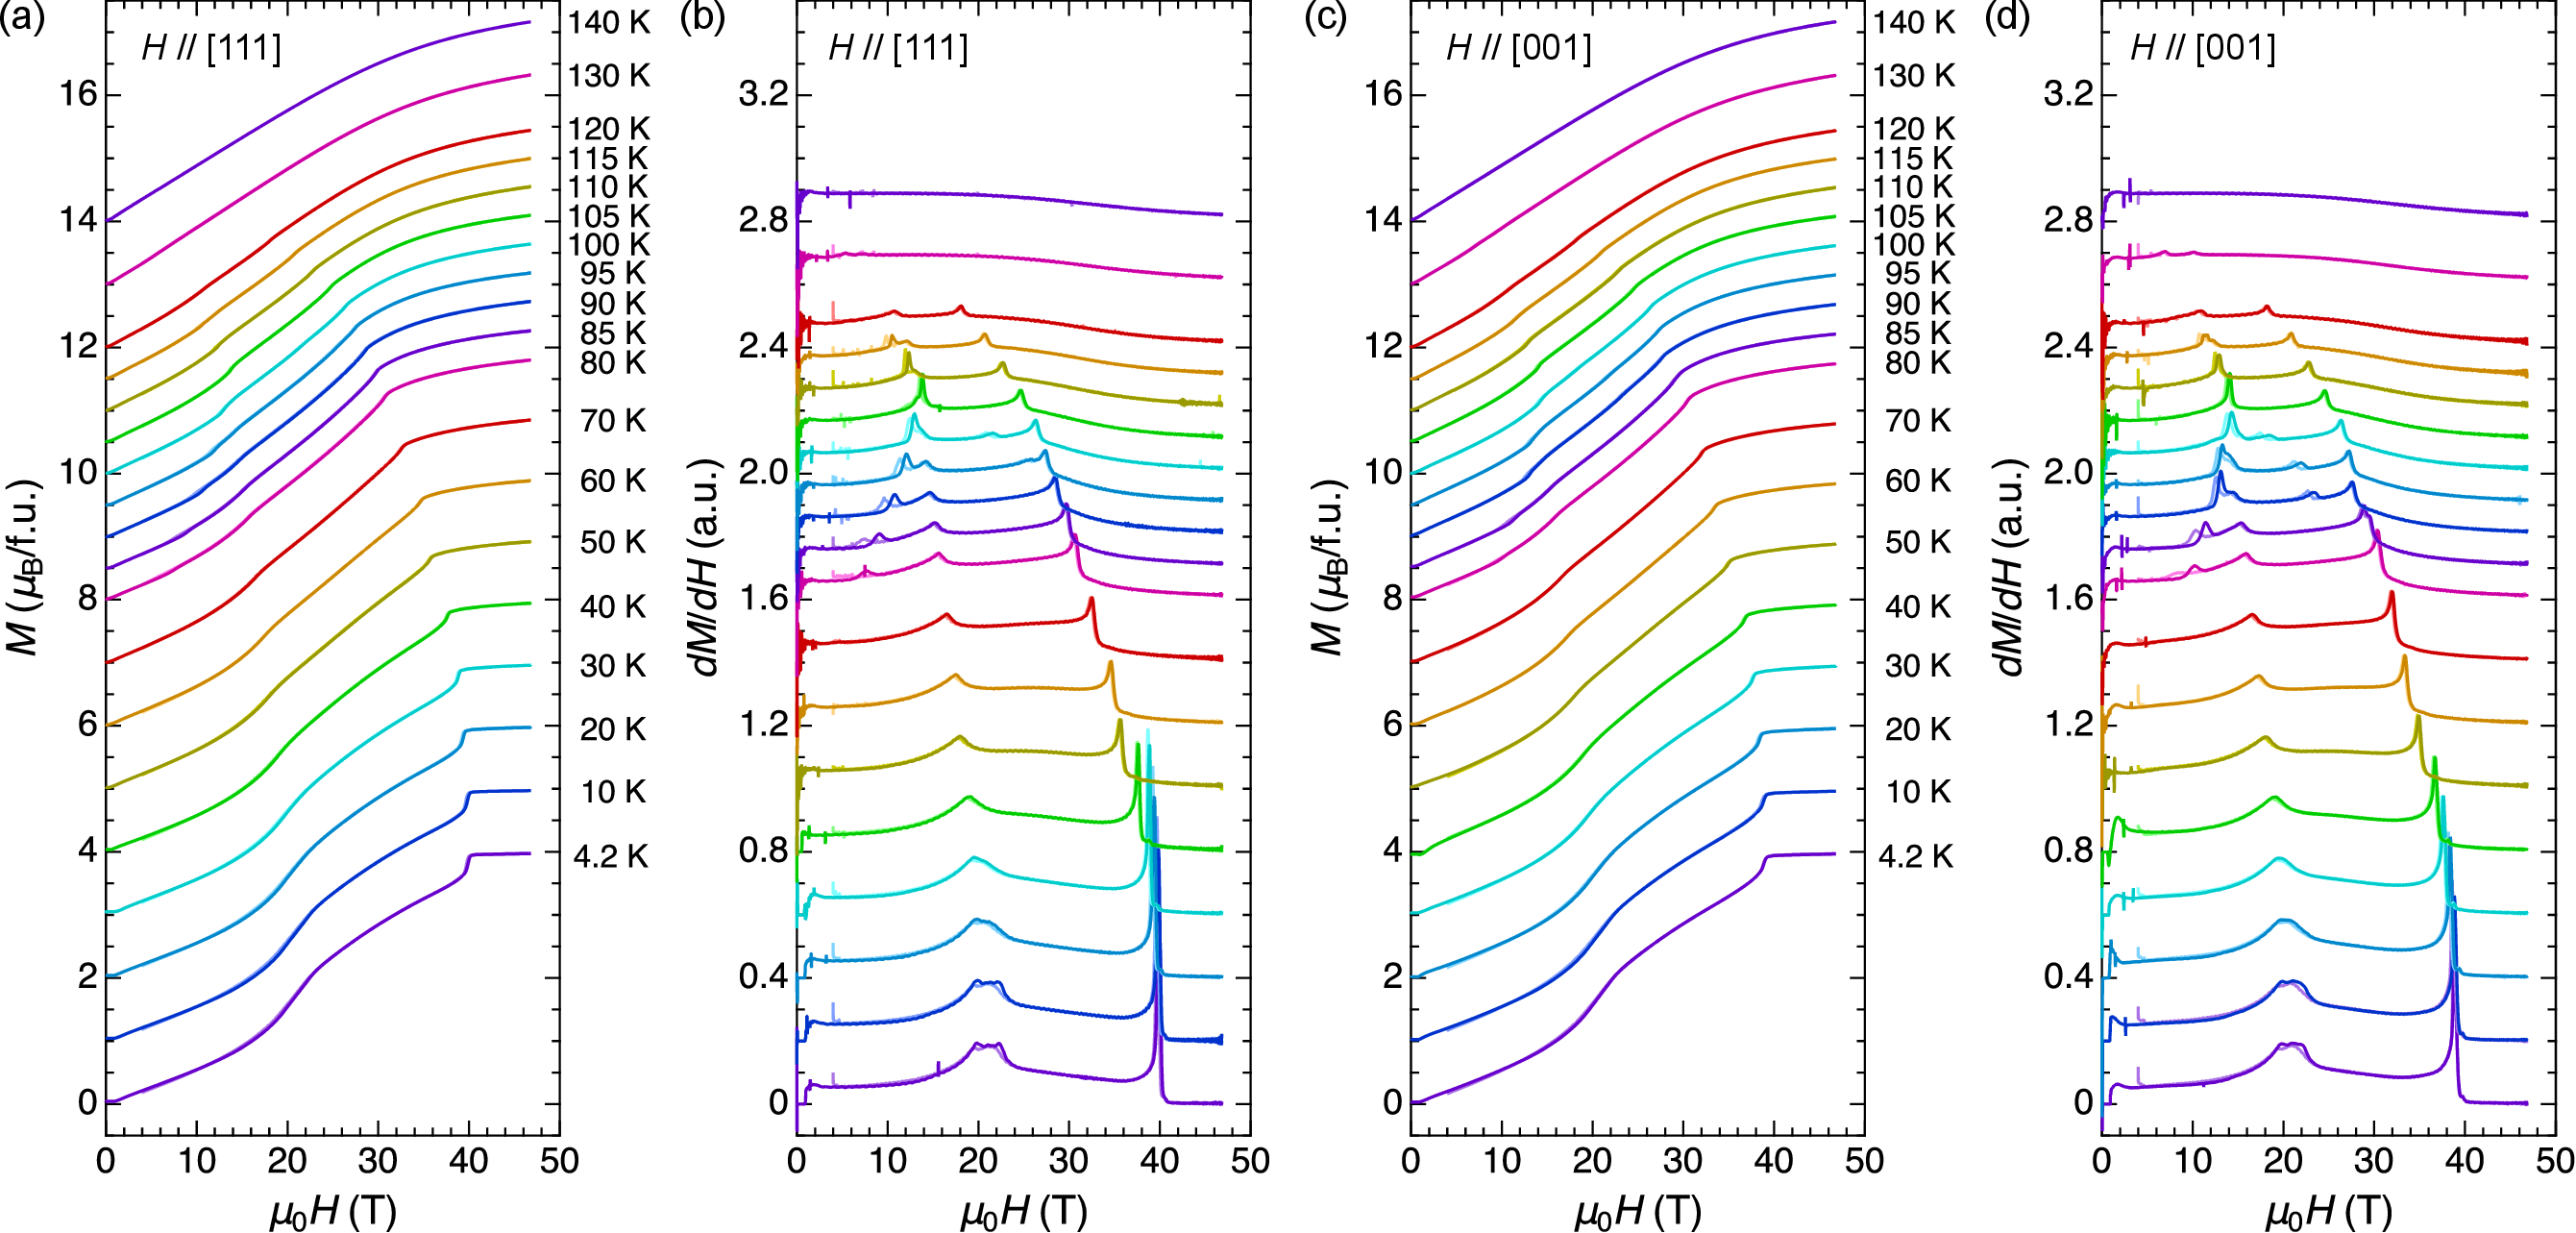}
\caption{Magnetic-field dependence of $M$ (a, c) and $dM/dH$ (b, d) measured at various temperature for $H \parallel [111]$ (a, b) and $H \parallel [001]$ (c, d). For clarity, the curves are vertically shifted except for $T = 4.2$~K. The data for the field-increasing (decreasing) process are shown in dark (light) colors.}
\label{FigS1}
\end{figure*}

\newpage
\subsection*{\label{Sec2} \large Note 2.~Additional magnetostriction data in pulsed high magnetic fields}
\vspace{+0.2cm}

Figure~\ref{FigS2} shows the field dependence of the longitudinal (left) and transverse (right) magnetostriction for $H \parallel [001]$ at various temperatures, measured simultaneously on the same single crystal.

\begin{figure*}[h]
\centering
\vspace{+1.0cm}
\includegraphics[width=0.5\linewidth]{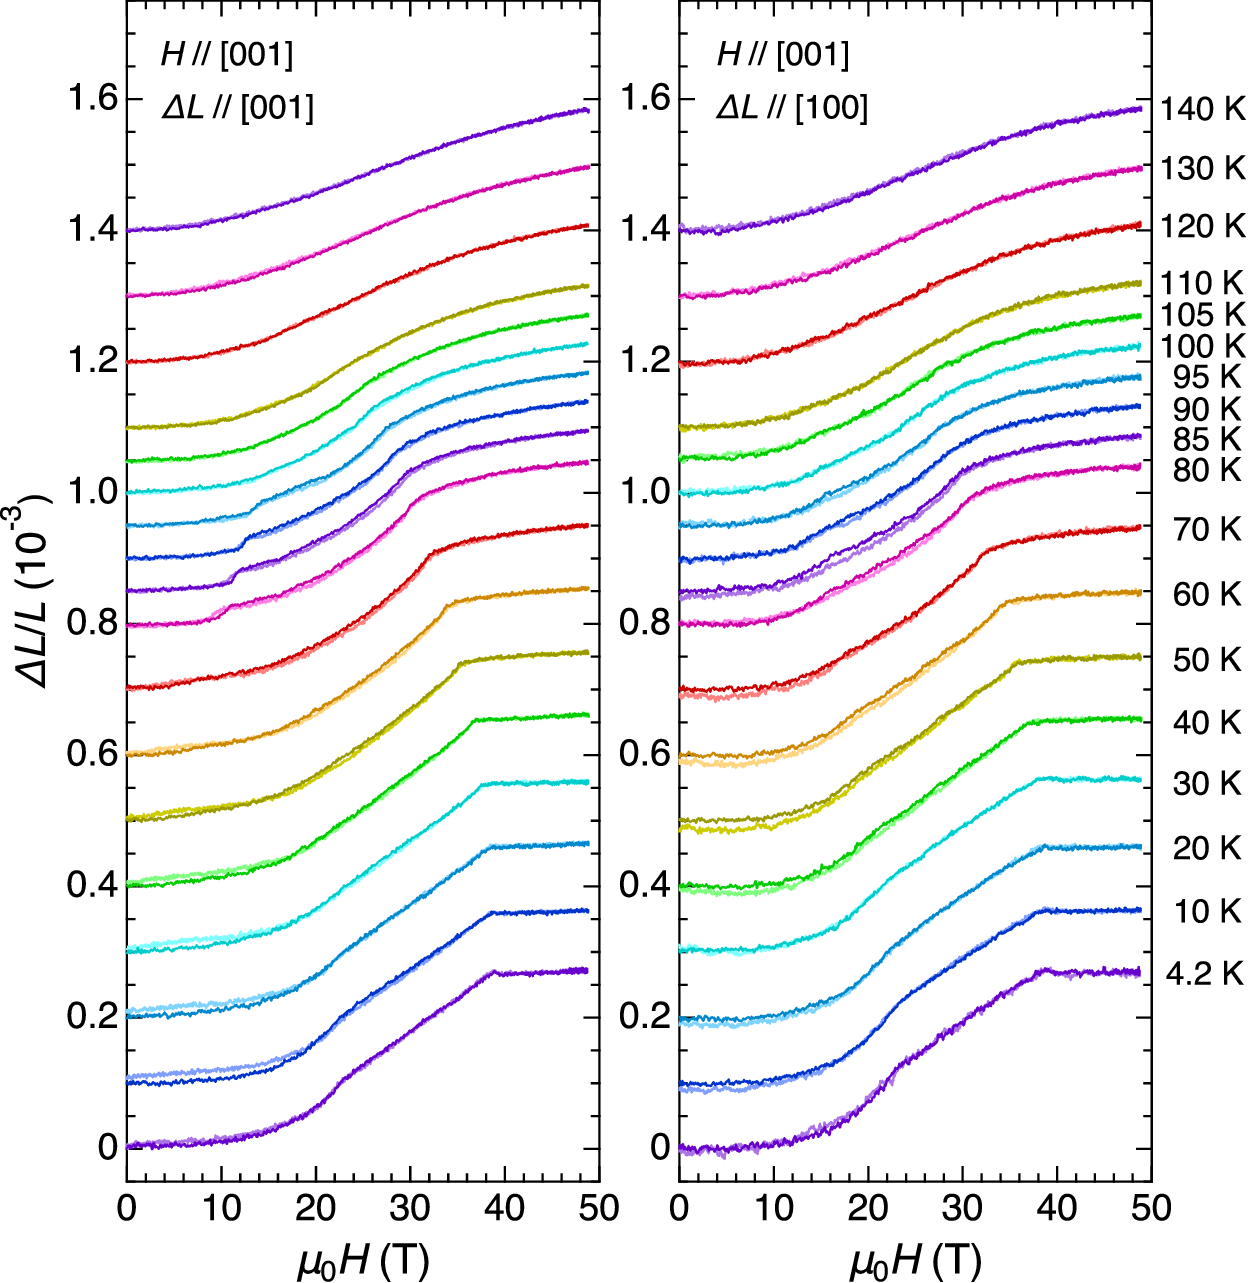}
\caption{Magnetic-field dependence of longitudinal (left) and transverse (right) magnetostriction measured at various temperature for $H \parallel [001]$. For clarity, the curves are vertically shifted except for $T = 4.2$~K. The data for the field-increasing (decreasing) process are shown in dark (light) colors.}
\label{FigS2}
\end{figure*}

\newpage
\subsection*{\label{Sec3} \large Note 3.~Additional ultrasound data in pulsed high magnetic fields}
\vspace{+0.2cm}

Figure~\ref{FigS3} compares the ultrasound data for ${\mathbf k} \parallel {\mathbf u} \parallel [111]$ and ${\mathbf k} \parallel {\mathbf u} \parallel [1{\overline 1}0]$.
The data in Fig.~\ref{FigS3}(a) are identical to those in Fig.~3(c) of the main text.

\begin{figure*}[h]
\centering
\vspace{+1.0cm}
\includegraphics[width=\linewidth]{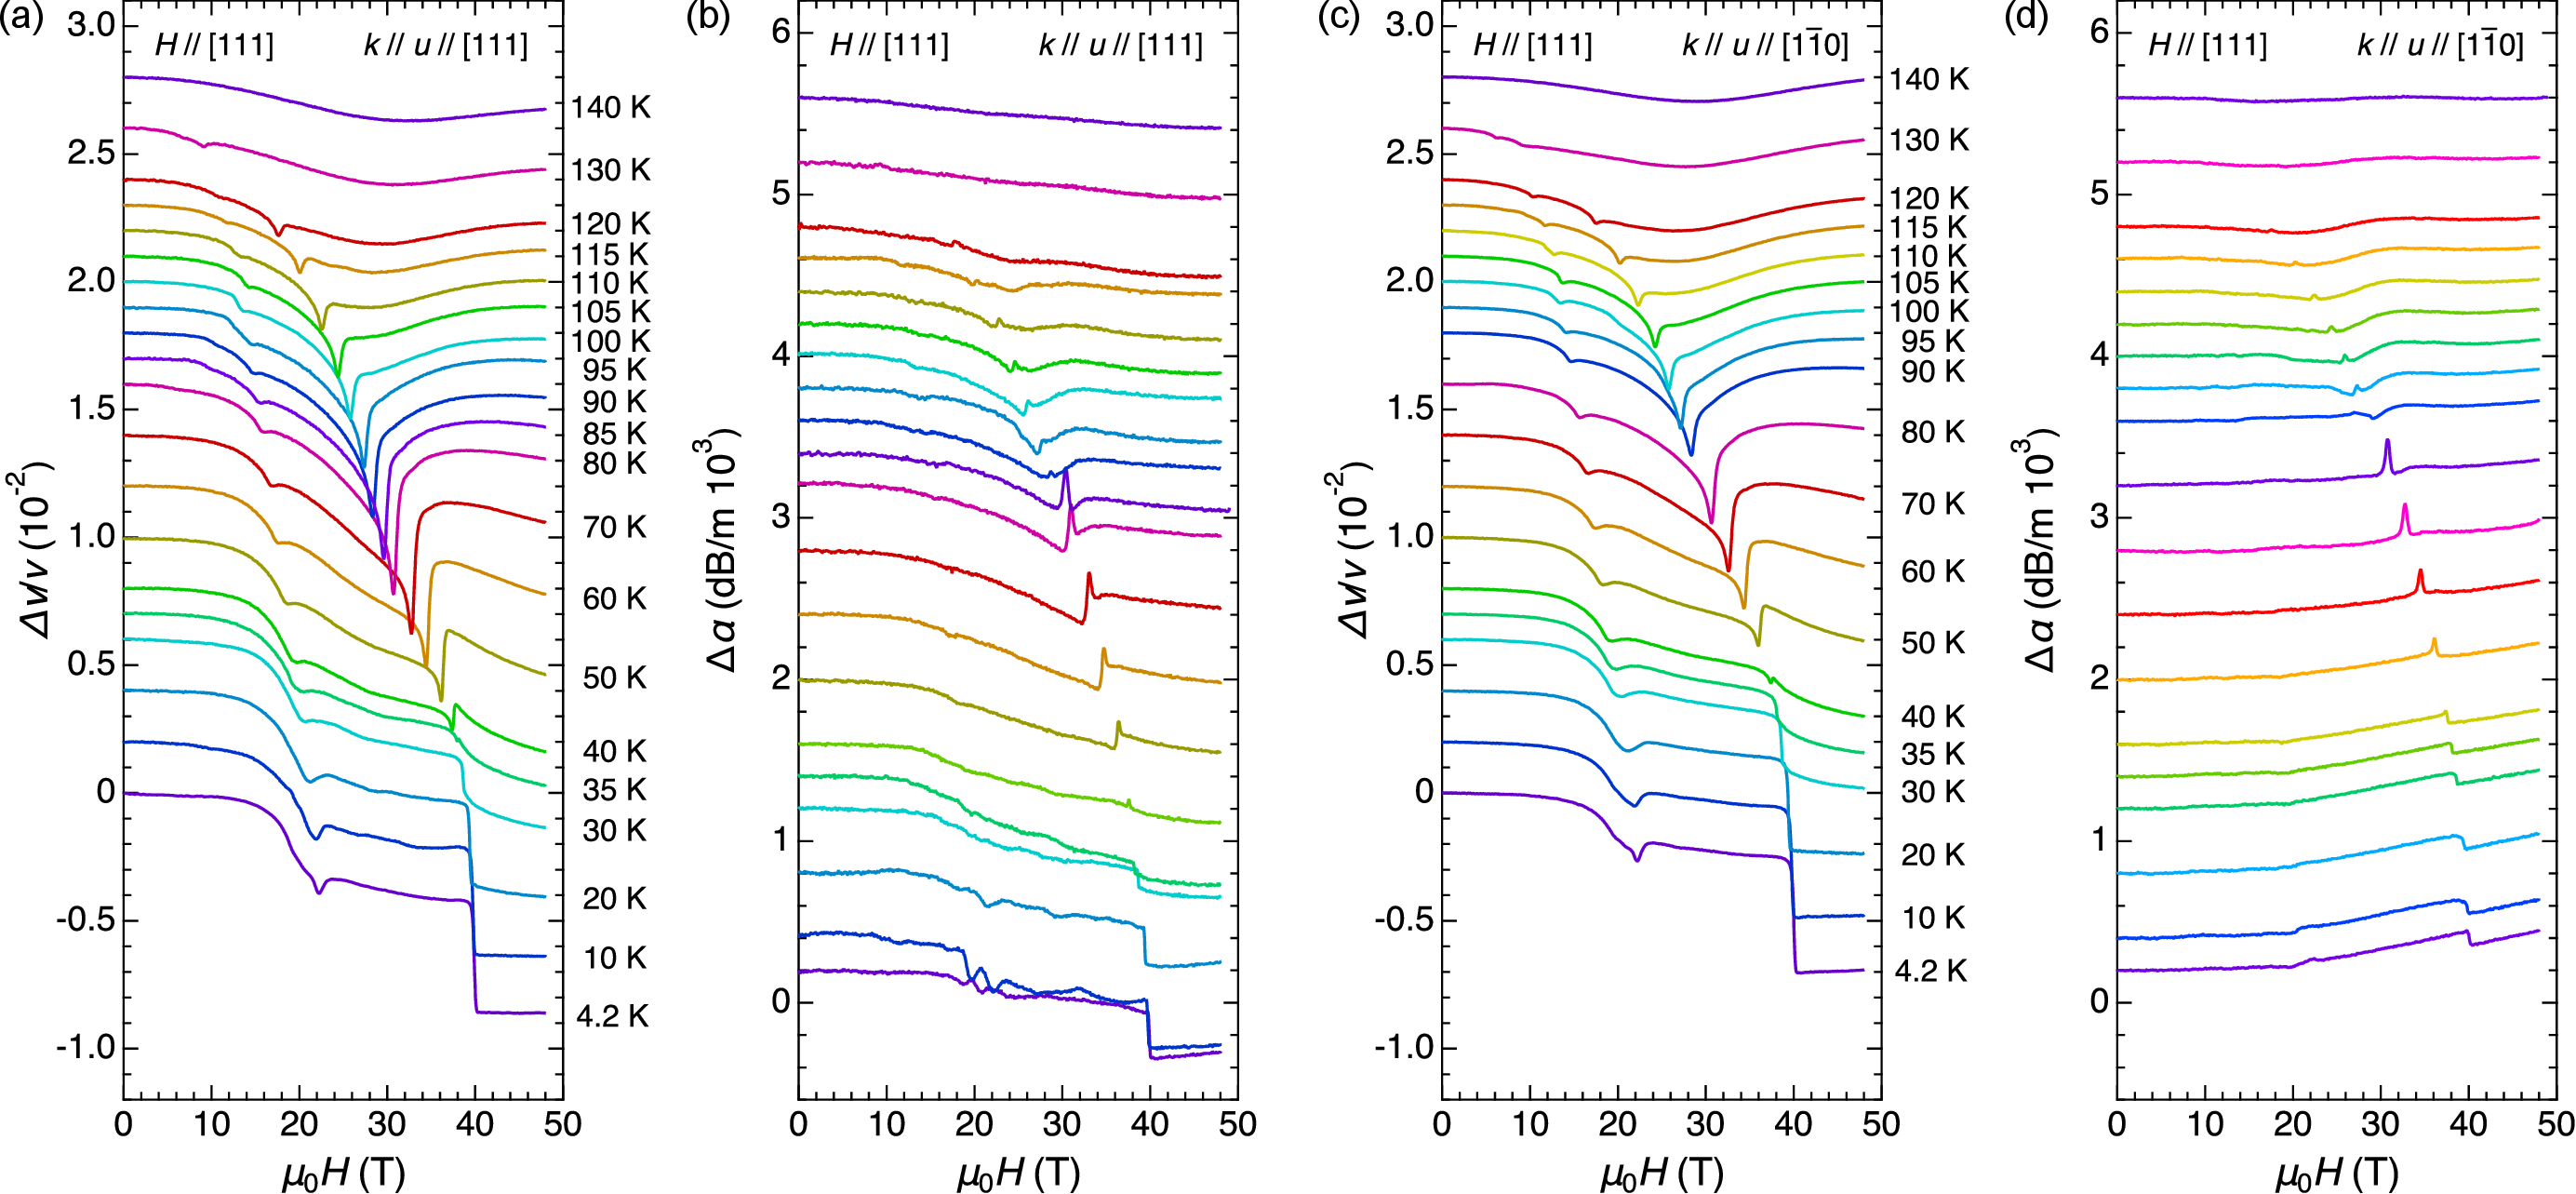}
\caption{Magnetic-field dependence of the longitudinal sound velocity (a, c) and attenuation (b, d) for ${\mathbf k} \parallel {\mathbf u} \parallel [111]$ (a, b)  and ${\mathbf k} \parallel {\mathbf u} \parallel [1{\overline 1}0]$ (c, d) measured at various temperature for $H \parallel [111]$. For clarity, the curves are vertically shifted except for $T = 4.2$~K. The data for the field-decreasing process are shown.}
\label{FigS3}
\end{figure*}

\newpage
\subsection*{\label{Sec4} \large Note 4.~Additional neutron scattering data under tilted magnetic fields}
\vspace{+0.2cm}

Figure~\ref{FigS4} shows neutron scattering profiles obtained from $\omega$ scans for the magnetic reflections at ${\mathbf Q}_{1} = (q, q, q)$, ${\mathbf Q}_{2} = (q, -q, -q)$, ${\mathbf Q}_{3} = (-q, q, -q)$, and ${\mathbf Q}_{4} = (-q, -q, q)$, where $q \approx 0.13$~r.l.u., measured while sweeping the magnetic field at 50~K after ZFC.
Although a triple-peak splitting has been reported in phase I \cite{2020_Ish}, it was observed here as a single broadened peak owing to the limited experimental resolution.
This interpretation is supported by the observation of a sharper single peak for the ${\mathbf Q}_{1}$ reflection in phase IV [Fig.~\ref{FigS4}(i)].

\begin{figure*}[h]
\centering
\vspace{+1.0cm}
\includegraphics[width=0.85\linewidth]{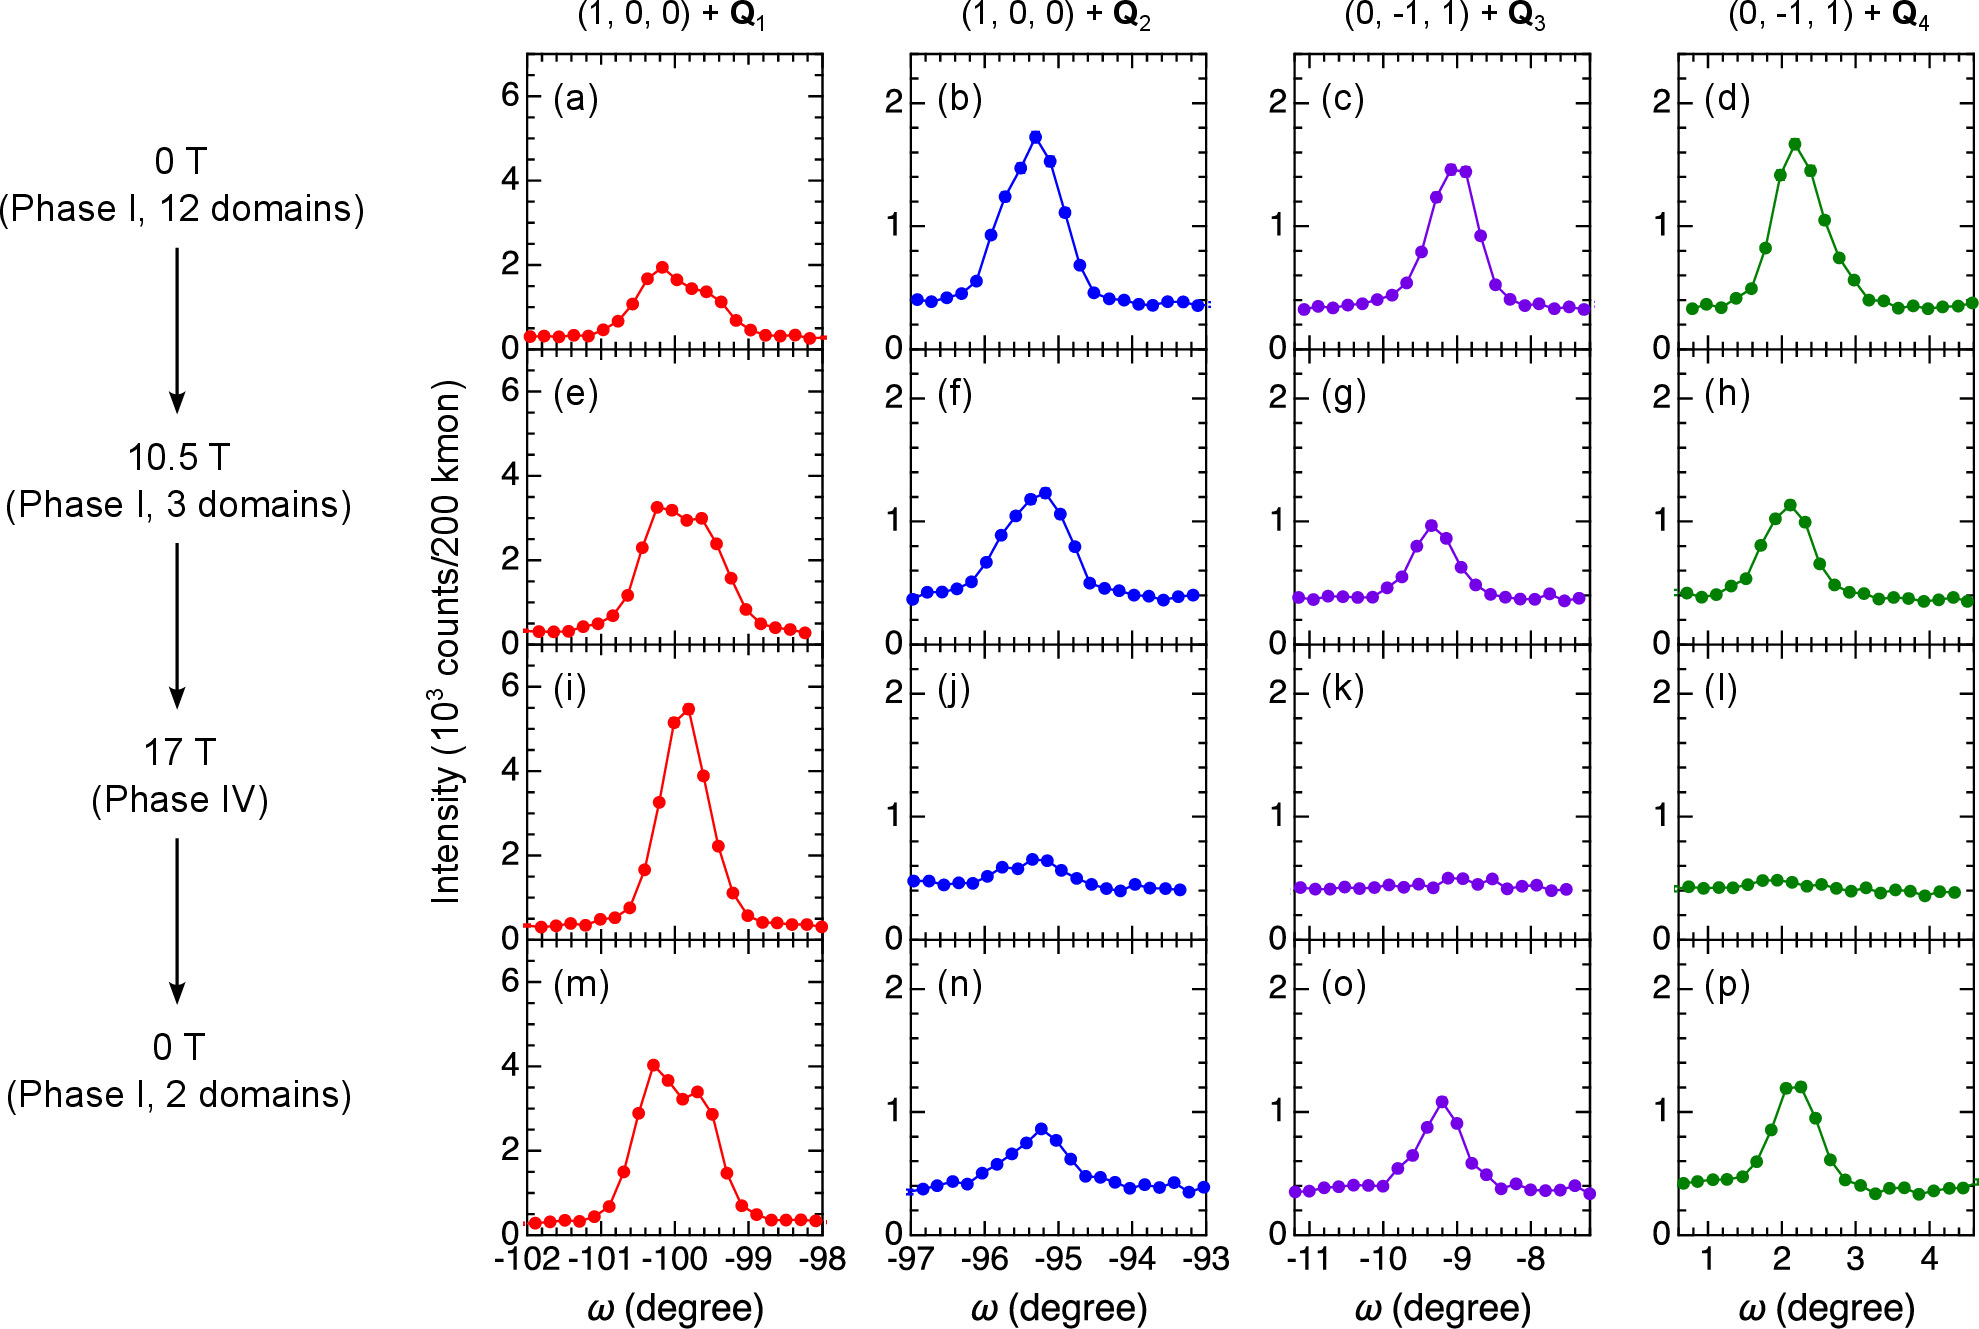}
\caption{Magnetic-field evolution of neutron scattering profiles obtained from $\omega$ scans for the magnetic reflections at ${\mathbf Q}_{1} = (q, q, q)$, ${\mathbf Q}_{2} = (q, -q, -q)$, ${\mathbf Q}_{3} = (-q, q, -q)$, and ${\mathbf Q}_{4} = (-q, -q, q)$ measured at 50~K after ZFC.}
\label{FigS4}
\end{figure*}

\newpage

We also performed single-crystal neutron scattering experiments at 110~K under tilted magnetic fields.
Figure~\ref{FigS5}(a) shows the field dependence of the integrated intensities of the ${\mathbf Q}_{1}$--${\mathbf Q}_{4}$ peaks measured at 110~K.
The corresponding neutron scattering profiles at 0~T (phase~II) and 10~T (phase~V) are shown in Figs.~\ref{FigS5}(b)--\ref{FigS5}(i).
As reported in Ref.~\cite{2020_Ish}, the magnetic structure in phase~II is a quadruple-${\mathbf Q}$ HL state, composed of a superposition of four equivalent helical modulations [Fig.~\ref{FigS5}(j)].
Upon entering phase~V, finite intensities are still observed for the ${\mathbf Q}_{2}$--${\mathbf Q}_{4}$ peaks, in contrast to phase~IV.
This observation suggests that phase~V is also a multiple-${\mathbf Q}$ state [Fig.~\ref{FigS5}(k)], although the number of superposed ${\mathbf Q}$ components cannot be determined from the present experiment.

\begin{figure*}[h]
\centering
\vspace{+1.0cm}
\includegraphics[width=\linewidth]{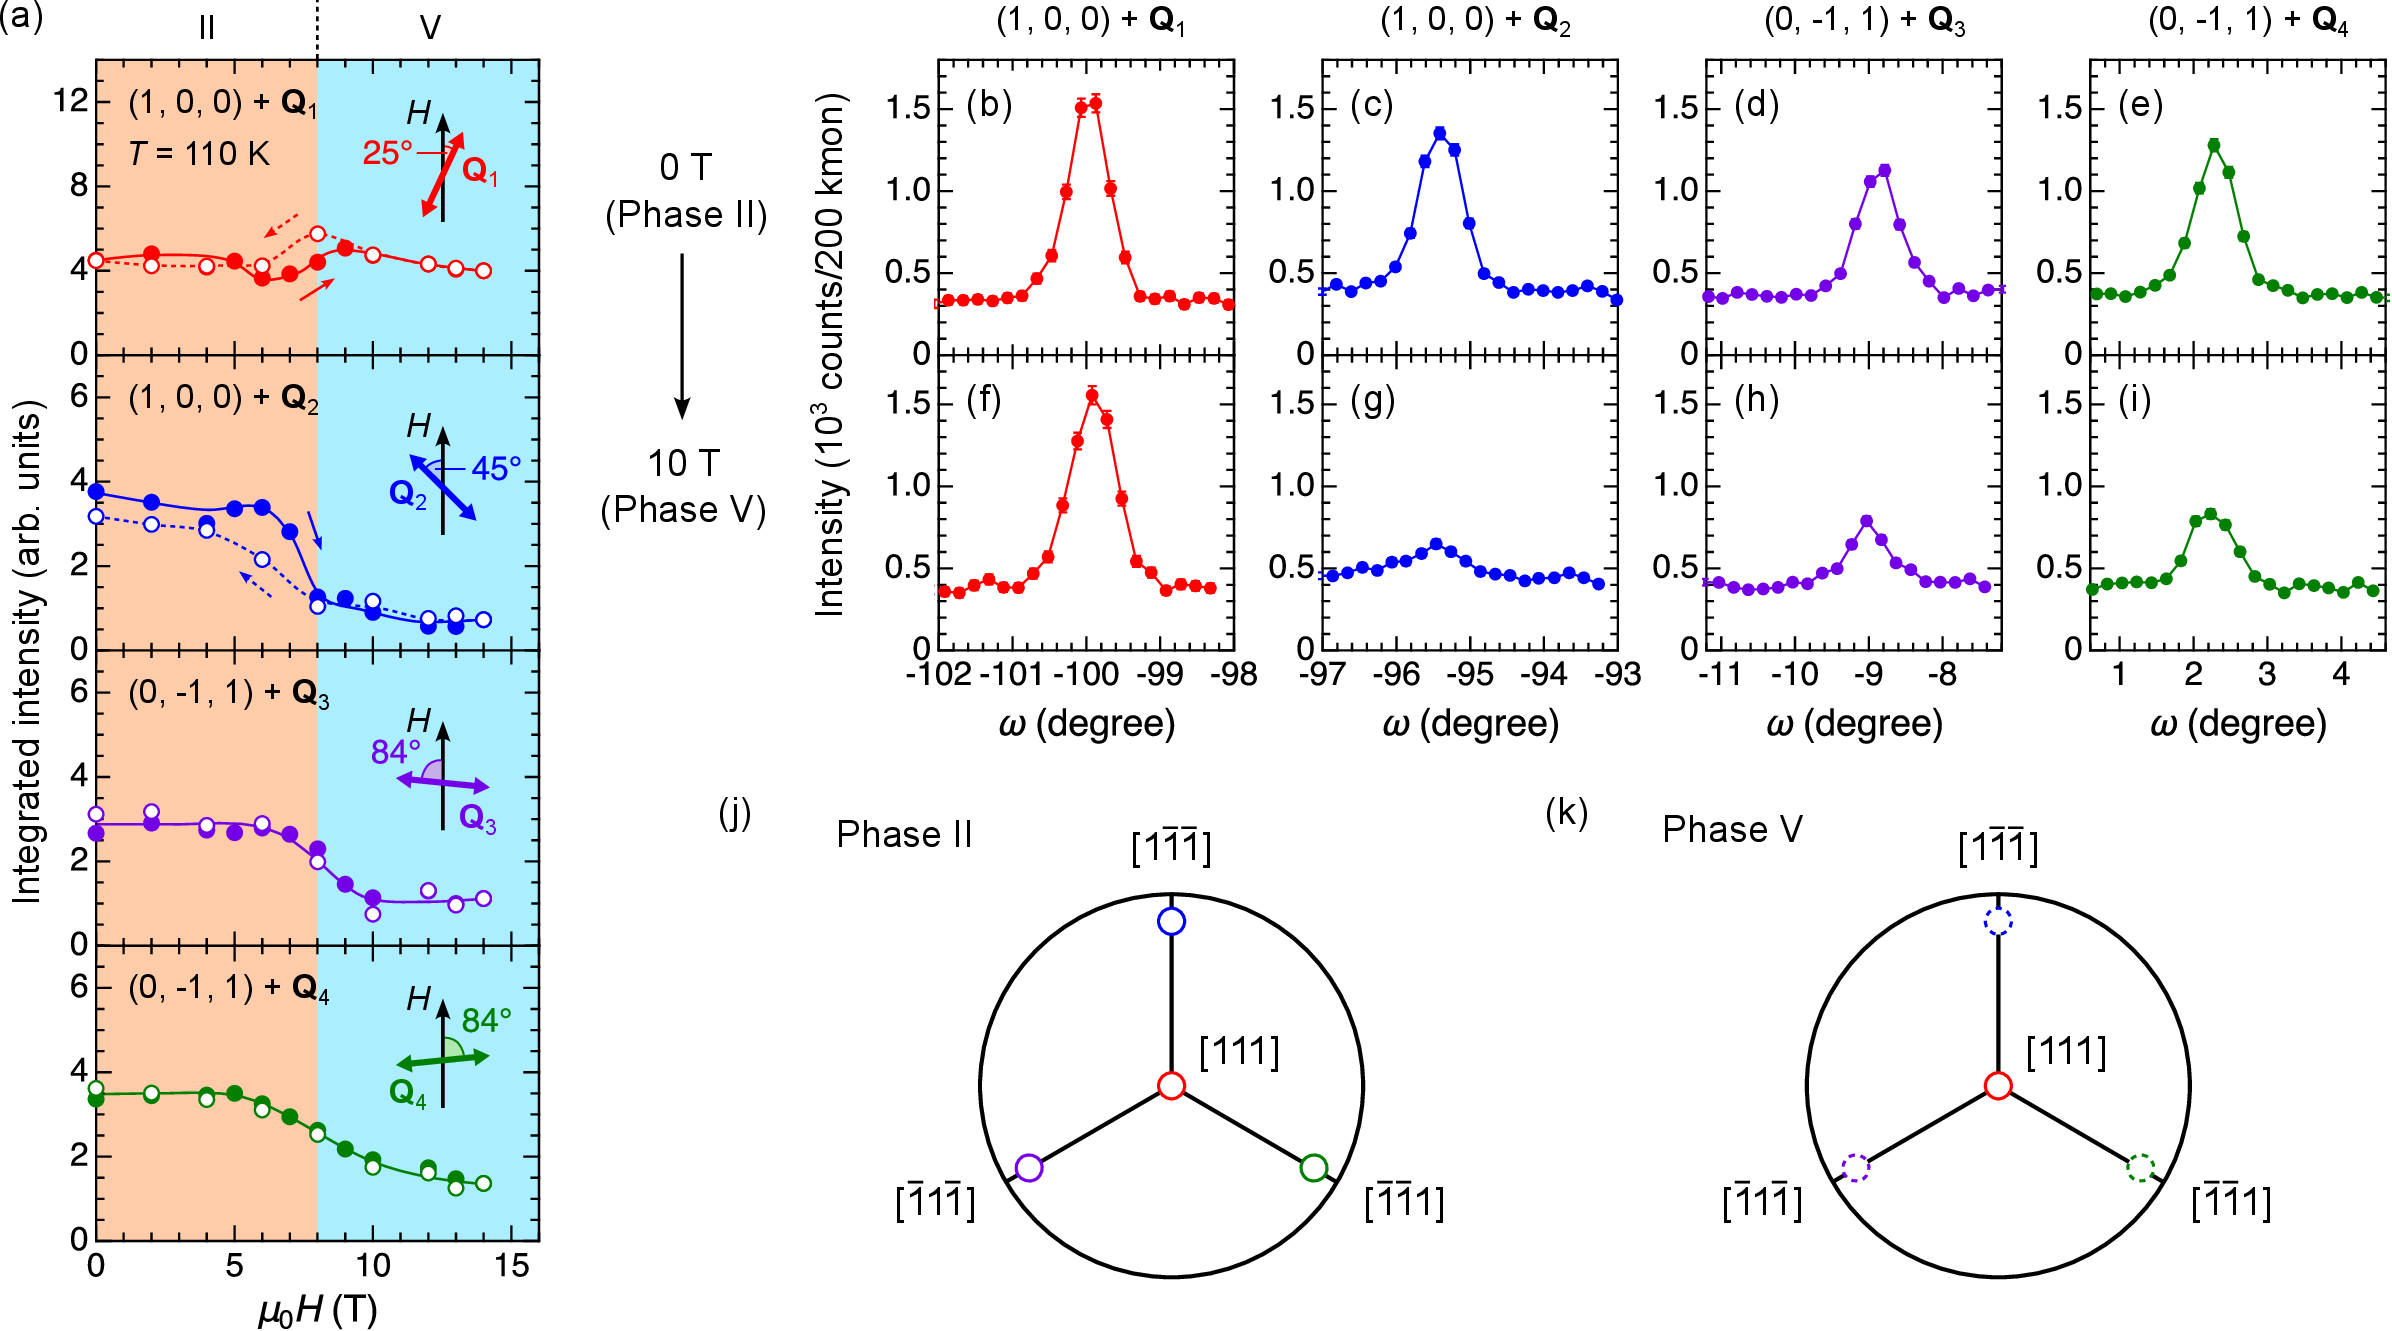}
\caption{(a) Magnetic-field dependence of the integrated intensities of the ${\mathbf Q}_{1}$--${\mathbf Q}_{4}$ peaks measured at 110~K. Data for the field-increasing (decreasing) process are plotted as filled (open) circles. The angle between each magnetic reflection vector and the applied field is shown in the inset of each panel. (b)--(i) Magnetic-field evolution of neutron scattering profiles obtained from $\omega$ scans for the magnetic reflections at ${\mathbf Q}_{1} = (q, q, q)$, ${\mathbf Q}_{2} = (q, -q, -q)$, ${\mathbf Q}_{3} = (-q, q, -q)$, and ${\mathbf Q}_{4} = (-q, -q, q)$. (j, k) Stereographic projections of magnetic scattering peaks at 0~T (j) and 10~T (k).}
\label{FigS5}
\end{figure*}

\newpage
\subsection*{\label{Sec5} \large Note 5.~Magnetic structure of 4{\it Q}-IFC phase}
\vspace{+0.2cm}

Figure~\ref{FigS6} illustrates the magnetic structure of the theoretically proposed 4{\it Q}-IFC phase (see Fig.~5 of the main text).
This magnetic structure is composed of a superposition of one helical and three sinusoidal modulations.
We propose that the newly discovered phase~VI in SrFeO$_{3}$ may correspond to 4{\it Q}-IFC phase.

\begin{figure*}[h]
\centering
\vspace{+1.0cm}
\includegraphics[width=0.6\linewidth]{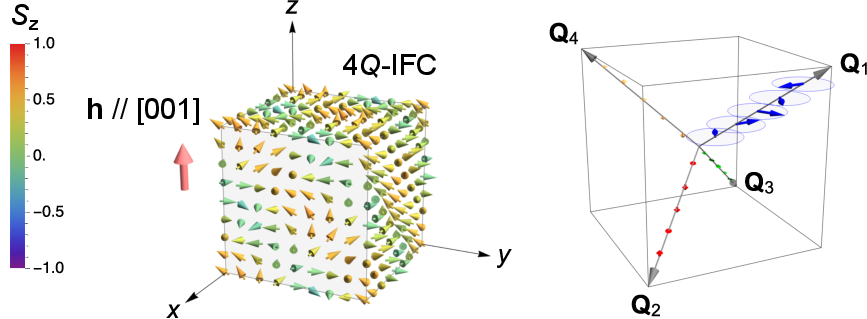}
\caption{Spin texture (left) and constituent waves (right) for the 4{\it Q}-IFC phase. The color bar represents the spin $z$ component, which is parallel to the field direction.}
\label{FigS6}
\end{figure*}

\hspace{+1.0cm}

\end{document}
